# Supplementary material for: Exotic aromatic B-series for the study of long time integrators for a class of ergodic SDEs
Source: arXiv:1707.02877 source file (2019-07-01)
Supplement: Supplementary file 1 [file Appendix_3.tex]

The use of trees becomes even more practical when the calculus are long. Here are the conditions of order 3.\\
We obtain $A_2\phi=F(\gamma_2)$ where
\begin{align*}
\gamma_2=&
\sum b_i a_{ij}c_j \etree 4 1 0 1
+\frac{\sigma^2}{2} \sum b_i a_{ij} \overline{c_j}^2 \etree 3 1 1 1
+\frac{1}{2} \sum b_i c_i^2 \etree 4 2 0 1
+\sigma^2 \sum b_i \overline{c_i} a_{ij} \overline{c_j} \etree 3 1 1 2
+\frac{\sigma^2}{2} \sum b_i c_i \overline{c_i}^2 \etree 3 1 1 3\\
&+\frac{\sigma^4}{8} \sum b_i \overline{c_i}^4 \etree 2 1 2 5
+\frac{\sigma^2}{2}\left(\sum b_i \overline{c_i}\right)^2 \etree 3 2 1 2
+\sigma^2 \sum b_i a_{ij} \overline{c_j} \etree 3 1 1 4
+\sigma^2 \sum b_i c_i \overline{c_i} \etree 3 1 1 5\\
&+\frac{\sigma^4}{2} \sum b_i \overline{c_i}^3 \etree 2 1 2 4
+\left(\sum b_i\right)\left(\sum b_i c_i\right) \etree 4 3 0 1
+\frac{\sigma^2}{2} \left(\sum b_i\right)\left(\sum b_i \overline{c_i}^2 \right) \etree 3 2 1 1\\
&+\frac{1}{6} \left(\sum b_i\right)^3 \etree 4 4 0 1
+\frac{\sigma^2}{2} \sum b_i c_i \etree 3 1 1 6
+\frac{\sigma^4}{4} \sum b_i \overline{c_i}^2 \etree 2 1 2 1
+\frac{\sigma^4}{2} \sum b_i \overline{c_i}^2 \etree 2 1 2 2\\
&+\sigma^2 \left(\sum b_i\right) \left(\sum b_i \overline{c_i} \right) \etree 3 2 1 3
+\frac{\sigma^4}{2} \sum b_i \overline{c_i} \etree 2 1 2 6
+\frac{\sigma^2}{4} \left(\sum b_i\right)^2 \etree 3 2 1 4\\
&+\frac{\sigma^4}{8} \left(\sum b_i\right) \etree 2 1 2 7
+\frac{\sigma^6}{48} \etree 1 1 3 1.
\end{align*}
~
If we suppose $\sum b_i=1$, then by integrating by part, we get
\begin{align*}
\gamma_2 &\sim \left(\sum b_i a_{ij}c_j-2\sum b_i a_{ij}\overline{c_j}+\sum b_i c_i-\left(\sum b_i \overline{c_i}\right)^2 \right) \etree 4 1 0 1\\
&+\frac{\sigma^2}{2}\left(\sum b_i a_{ij}\overline{c_j}^2-2\sum b_i a_{ij}\overline{c_j}+\sum b_i c_i-\left(\sum b_i \overline{c_i}\right)^2 \right) \etree 3 1 1 1\\
&+\left(\frac{1}{2}\sum b_i c_i^2 -2\sum b_i \overline{c_i}c_i-2\sum b_i \overline{c_i} +2\sum b_i \overline{c_i}^2 +\frac{1}{3} + \sum b_i c_i\right) \etree 4 2 0 1\\
&+\sigma^2\left(\sum b_i \overline{c_i} a_{ij}\overline{c_j}-\sum b_i c_i\overline{c_i}-\sum b_i \overline{c_i}+\sum b_i \overline{c_i}^2+\frac{1}{6}+\sum b_i c_i\right.\\
&\left.-\sum b_i a_{ij}\overline{c_j}-\frac{1}{2}\left(\sum b_i \overline{c_i}\right)^2 \right) \etree 3 1 1 2\\
&+\sigma^2\left(\frac{1}{2}\sum b_i c_i\overline{c_i}^2-\sum b_i\overline{c_i}^3-2\sum b_i \overline{c_i}+\frac{5}{2}\sum b_i \overline{c_i}^2-\sum b_i c_i\overline{c_i}+\frac{1}{2}\sum b_i c_i+\frac{1}{3} \right) \etree 3 1 1 3\\
&+\sigma^4\left(\frac{1}{8}\sum b_i \overline{c_i}^4-\frac{1}{2}\sum b_i\overline{c_i}^3-\frac{1}{2}\sum b_i \overline{c_i}+\frac{3}{4}\sum b_i \overline{c_i}^2+\frac{1}{12} \right) \etree 2 1 2 5 .
\end{align*}
