# Supplementary material for: Exotic aromatic B-series for the study of long time integrators for a class of ergodic SDEs
Source: arXiv:1707.02877 source file (2019-07-01)
Supplement: Supplementary file 2 [file Appendix_equivariance.tex]

\label{appendix:isometric_equivariance}
\begin{proof}[Proof of Theorem \ref{theorem:equivariance}]
By an argument of linearity, it suffices to prove the $\Or_d(\R)$-equivariance of each exotic aromatic forests.
Let $\gamma=(V,E,L)$ be an exotic aromatic rooted forest, $f$ a smooth function. We name $r$ the root and $V^0=V\smallsetminus\{r\}=\{v_1,\dots ,v_m\}$ the other nodes. We denote $l_1$,\dots ,$l_s$ the elements of $L$.
Then
$$F(\gamma)(f)=\sum_{i_{v_1},\dots ,i_{v_m}=1}^d \sum_{j_{l_1},\dots ,j_{l_s}=1}^d \left(\prod_{v\in V^0} \partial_{I_{\pi(v)}} \partial_{J_{\Gamma(v)}} f_{i_v}\right) \partial_{I_{\pi(r)}} \partial_{J_{\Gamma(r)}} f.$$
Let $A\in\Or_d(\R)$ and $x\in \R^d$, we would like to prove that
\begin{equation}
\label{equation:goal_equivariance_proof}
F(\gamma)(A*f)(x)=(F(\gamma)(Af(A^{-1}.)))(x)=A(F(\gamma)(f))(A^{-1}x).
\end{equation}
On the first hand, we have
\begin{align*}
(F(\gamma)(A*f))_{j_0}(x) &=
\sum_{i_{v_1},\dots ,i_{v_m}=1}^d \sum_{j_{l_1},\dots ,j_{l_s}=1}^d\\
&\left(\prod_{v\in V^0} \sum_{k=1}^d \sum_{P_{\pi(v)},Q_{\Gamma(v)}} a_{i_v,k} . a_{I_{\pi(v)},P_{\pi(v)}} . a_{J_{\Gamma(v)},Q_{\Gamma(v)}} \partial_{P_{\pi(v)}} \partial_{Q_{\Gamma(v)}} f_{k}\right)(A^{-1}x)\\
&\cdot \left(\sum_{k=1}^d \sum_{P_{\pi(r)},Q_{\Gamma(r)}} a_{j_0,k} . a_{I_{\pi(r)},P_{\pi(r)}} . a_{J_{\Gamma(r)},Q_{\Gamma(r)}} \partial_{P_{\pi(r)}} \partial_{Q_{\Gamma(r)}} f_{k}\right)(A^{-1}x),
\end{align*}
where we define $a_{I,J}:=\prod_{i\in I,j\in J} a_{i,j}$ and $$\sum_{P_{\pi(v)},Q_{\Gamma(v)}}:=\sum_{v'\in\pi(v),l'\in\Gamma(v)} \sum_{p_{v'}=1}^d \sum_{q_{l'}=1}^d.$$

\paragraph*{First step: simplification of edges.}
For each edge of the form $(v,v')$, the following sum appears
$$\sum_{i_{v},k,p_{v}} a_{i_{v},k}.a_{i_{v},p_{v}}(\partial_{p_{v}}g_{l})h_k=\sum_{p_{v}}(\partial_{p_{v}}g_{l})h_{p_{v}},$$
where $g$ and $h$ are certain derivatives of $f$, and where we used the isometric property of $A$.
Thus, we can simplify our expression into
\begin{align*}
(F(\gamma)(A*f))_{j_0}(x)&=
\sum_{p_{v_1},\dots ,p_{v_m}=1}^d \sum_{j_{l_1},\dots ,j_{l_s}=1}^d\\
&\left(\prod_{v\in V^0} \sum_{Q_{\Gamma(v)}} a_{J_{\Gamma(v)},Q_{\Gamma(v)}} \partial_{P_{\pi(v)}} \partial_{Q_{\Gamma(v)}} f_{p_v}\right)(A^{-1}x)\\
&\cdot \left(\sum_{k=1}^d \sum_{Q_{\Gamma(r)}} a_{j_0,k} . a_{J_{\Gamma(r)},Q_{\Gamma(r)}} \partial_{P_{\pi(r)}} \partial_{Q_{\Gamma(r)}} f_{k}\right)(A^{-1}x).
\end{align*}

\paragraph*{Second step: simplification of lianas.}
This is the part where we need $A$ to be isometric.
If $l$ is a liana linking $v$ and $v'$, then the following sum appears
$$\sum_{j_l,q_l,q_l'} a_{j_l,q_l} (\partial_{q_l} g_{p_v})a_{j_l,q_l'} (\partial_{q_l'} h_{p_{v'}})=\sum_{q_l} (\partial_{q_l} g_{p_v})(\partial_{q_l} h_{p_{v'}})$$
where $g$ and $h$ are certain derivatives of $f$.
Notice that the number of sums over indexes of the form $q_l$ is two times the number of lianas, and we identify those pairs of sums according to lianas.
Finally we have 
\begin{align*}
(F(\gamma)(A*f))_{j_0}(x)&=
\sum_{p_{v_1},\dots ,p_{v_m}=1}^d \sum_{q_{l_1},\dots ,q_{l_s}=1}^d\\
&\left(\prod_{v\in V^0} \partial_{P_{\pi(v)}} \partial_{Q_{\Gamma(v)}} f_{p_v}\right)(A^{-1}x)\\
&\cdot \left(\sum_{k=1}^d a_{j_0,k} \partial_{P_{\pi(r)}} \partial_{Q_{\Gamma(r)}} f_{k}\right)(A^{-1}x).
\end{align*}
This shows \eqref{equation:goal_equivariance_proof}, and thus we obtain equivariance.
\end{proof}

Notice that we do not need $A$ to be isometric to write the first step of the proof, $A$ invertible is enough. If we do not suppose $A$ isometric, the term $a_{I_{\pi(v)},P_{\pi(v)}}$ becomes $b_{P_{\pi(v)},I_{\pi(v)}}$, where $B=A^{-1}$, and the sums still simplify. Thus the first step proves the affine equivariance of aromatic B-series methods.
