# Supplementary material for: Exotic aromatic B-series for the study of long time integrators for a class of ergodic SDEs
Source: arXiv:1707.02877 source file (2019-07-01)
Supplement: Supplementary file 3 [file Appendix_1.tex]

\subsection*{Isometric equivariance of $\Phi(f)=\Id+f'(\Delta f)$}

We saw the $\Or_d(\R)\ltimes \R^d$-equivariance of $\Phi$ is the same as the $\Or_d(\R)\times \{0\}$-equivariance of $\Phi_0(f)=f'(\Delta f)$.
We take $A=(a_{i,j})_{i,j}\in \GL_d(\R)$, then
$$f'(\Delta f)=\sum_i \sum_j \partial_{x_j,x_j} f_i. \partial_{x_i} f.$$
We develop $\Phi_0 (A*f)$.
\begin{align*}
\Phi_0 (A*f)_{j_0}(x)&=\sum_i \sum_j \partial_{x_j,x_j} (A*f)_i . \partial_{x_i} (A*f)_{j_0}\\
&=\sum_i \sum_j \left( \sum_{k'} \sum_{q_1,q_2} a_{i,k'} a_{j,q_1} a_{j,q_2} \partial_{x_{q_1},x_{q_2}} f_{k'} (A^{-1}x) \right)\\
&\quad \times \left( \sum_k \sum_p a_{j_0,k} a_{i,p} \partial_{x_p} f_k (A^{-1}x)\right)\\
&=\sum_p \sum_{q_1,q_2} \sum_{k'} \left(\sum_i a_{i,k'} a_{i,p}\right)\times \left(\sum_j a_{j,q_1} a_{j,q_2}\right)\\
&\quad \times \left(\partial_{x_{q_1},x_{q_2}} f_{k'} (A^{-1}x) \sum_k a_{j_0,k} \partial_{x_p} f_k (A^{-1}x)\right)\\
&=\sum_p \sum_{q_1} \partial_{x_{q_1},x_{q_1}} f_{p} (A^{-1}x) \sum_k a_{j_0,k} \partial_{x_p} f_k (A^{-1}x)\\
&=(A\Phi_0 f)_{j_0}(A^{-1}x)
\end{align*}
Thus $\Phi_0$ is isometric equivariant.
