# Supplementary material for: Exotic aromatic B-series for the study of long time integrators for a class of ergodic SDEs
Source: arXiv:1707.02877 source file (2019-07-01)
Supplement: Supplementary file 4 [file Appendix_2.tex]

1 1 0 1 $\etree 1 1 0 1$\\
1 1 1 1 $\etree 1 1 1 1$\\
1 1 2 1 $\etree 1 1 2 1$\\
1 1 3 1 $\etree 1 1 3 1$\\
1 2 0 1 $\etree 1 2 0 1$\\
2 1 0 1 $\etree 2 1 0 1$\\
2 1 1 1 $\etree 2 1 1 1$\\
2 1 1 2 $\etree 2 1 1 2$\\
2 1 1 3 $\etree 2 1 1 3$\\
2 1 2 1 $\etree 2 1 2 1$\\
2 1 2 2 $\etree 2 1 2 2$\\
2 1 2 3 $\etree 2 1 2 3$\\
2 1 2 4 $\etree 2 1 2 4$\\
2 1 2 5 $\etree 2 1 2 5$\\
2 1 2 6 $\etree 2 1 2 6$\\
2 1 2 7 $\etree 2 1 2 7$\\
2 2 0 1 $\etree 2 2 0 1$\\
3 1 0 1 $\etree 3 1 0 1$\\
3 1 1 1 $\etree 3 1 1 1$\\
3 1 1 2 $\etree 3 1 1 2$\\
3 1 1 3 $\etree 3 1 1 3$\\
3 1 1 4 $\etree 3 1 1 4$\\
3 1 1 5 $\etree 3 1 1 5$\\
3 1 1 6 $\etree 3 1 1 6$\\
3 2 0 1 $\etree 3 2 0 1$\\
3 2 1 1 $\etree 3 2 1 1$\\
3 2 1 2 $\etree 3 2 1 2$\\
3 2 1 3 $\etree 3 2 1 3$\\
3 2 1 4 $\etree 3 2 1 4$\\
4 1 0 1 $\etree 4 1 0 1$\\
4 2 0 1 $\etree 4 2 0 1$\\
4 3 0 1 $\etree 4 3 0 1$\\
4 4 0 1 $\etree 4 4 0 1$\\
5 2 0 1 $\etree 5 2 0 1$\\
5 2 0 2 $\etree 5 2 0 2$\\
